# Supplementary material for: Band Gap and Edge Engineering via Ferroic Distortion and Anisotropic Strain: The Case of SrTiO$_{3}$
Source: arXiv:1109.1271 source file (2011-09-06)
Supplement: Supplementary file 1 [file berger11_supp.pdf]

# Supplemental Information: Band Gap and Edge Engineering via Ferroic Distortion and Anisotropic Strain: The Case of $SrTiO_3$

Robert F. Berger,[1] Craig J. Fennie,[2] and Jeffrey B. Neaton[1,*]

[1] *Molecular Foundry, Lawrence Berkeley National Laboratory, Berkeley, CA*
[2] *School of Applied and Engineering Physics, Cornell University, Ithaca, NY*

(Dated: June 9, 2011)

PACS numbers:

---

* Electronic address: jbneaton@lbl.gov

TABLE I: Structural parameters of STO under biaxial strain perpendicular to [001], optimized in DFT-LDA using VASP. These parameters do not fully specify all structures, nor do they reflect AFD supercells. FE amplitudes are expressed as average relative translations of Ti and O atoms, while AFD amplitudes are expressed as average translations of O atoms.

| Structure | Strain | $a$ (Å) | $c$ (Å) | FE amplitude (Å) | AFD amplitude (Å) |
|---|---|---|---|---|---|
| Paraelectric | -4.0% | 3.7096 | 3.9634 | | |
| | -3.5% | 3.7290 | 3.9497 | | |
| | -3.0% | 3.7483 | 3.9366 | | |
| | -2.5% | 3.7676 | 3.9237 | | |
| | -2.0% | 3.7869 | 3.9111 | | |
| | -1.5% | 3.8062 | 3.8989 | | |
| | -1.0% | 3.8256 | 3.8869 | | |
| | -0.5% | 3.8449 | 3.8754 | | |
| | 0.0% | 3.8642 | 3.8642 | | |
| | 0.5% | 3.8835 | 3.8532 | | |
| | 1.0% | 3.9028 | 3.8427 | | |
| | 1.5% | 3.9222 | 3.8323 | | |
| | 2.0% | 3.9415 | 3.8224 | | |
| | 2.5% | 3.9608 | 3.8129 | | |
| | 3.0% | 3.9801 | 3.8037 | | |
| | 3.5% | 3.9994 | 3.7947 | | |
| | 4.0% | 4.0188 | 3.7861 | | |
| FE[001] | -4.0% | 3.7096 | 4.0908 | 0.2485 | |
| | -3.5% | 3.7290 | 4.0389 | 0.2106 | |
| | -3.0% | 3.7483 | 3.9983 | 0.1775 | |
| | -2.5% | 3.7676 | 3.9665 | 0.1488 | |
| | -2.0% | 3.7869 | 3.9389 | 0.1208 | |
| | -1.5% | 3.8062 | 3.9156 | 0.0941 | |
| | -1.0% | 3.8256 | 3.8949 | 0.0651 | |
| | -0.5% | 3.8449 | 3.8771 | 0.0309 | |
| FE[110] | 0.5% | 3.8835 | 3.8528 | 0.0399 | |
| | 1.0% | 3.9028 | 3.8409 | 0.0845 | |
| | 1.5% | 3.9222 | 3.8285 | 0.1142 | |
| | 2.0% | 3.9415 | 3.8161 | 0.1391 | |
| | 2.5% | 3.9608 | 3.8038 | 0.1615 | |
| | 3.0% | 3.9801 | 3.7911 | 0.1823 | |
| | 3.5% | 3.9994 | 3.7786 | 0.2019 | |
| | 4.0% | 4.0188 | 3.7658 | 0.2207 | |
| AFD[001] | -4.0% | 3.7096 | 3.9952 | | 0.2356 |
| | -3.5% | 3.7290 | 3.9776 | | 0.2234 |
| | -3.0% | 3.7483 | 3.9609 | | 0.2113 |
| | -2.5% | 3.7676 | 3.9444 | | 0.1988 |
| | -2.0% | 3.7869 | 3.9287 | | 0.1860 |
| | -1.5% | 3.8062 | 3.9135 | | 0.1728 |
| | -1.0% | 3.8256 | 3.8991 | | 0.1599 |
| | -0.5% | 3.8449 | 3.8852 | | 0.1457 |
| | 0.0% | 3.8642 | 3.8718 | | 0.1315 |
| | 0.5% | 3.8835 | 3.8589 | | 0.1173 |
| | 1.0% | 3.9028 | 3.8467 | | 0.1004 |
| | 1.5% | 3.9222 | 3.8358 | | 0.0824 |
| | 2.0% | 3.9415 | 3.8240 | | 0.0627 |
| | 2.5% | 3.9608 | 3.8130 | | 0.0237 |
| AFD[110] | -4.0% | 3.7096 | 3.9593 | | 0.1629 |
| | -3.5% | 3.7290 | 3.9447 | | 0.1591 |
| | -3.0% | 3.7483 | 3.9305 | | 0.1563 |
| | -2.5% | 3.7676 | 3.9167 | | 0.1556 |
| | -2.0% | 3.7869 | 3.9032 | | 0.1562 |
| | -1.5% | 3.8062 | 3.8904 | | 0.1556 |
| | -1.0% | 3.8256 | 3.8776 | | 0.1580 |
| | -0.5% | 3.8449 | 3.8651 | | 0.1603 |
| | 0.0% | 3.8642 | 3.8534 | | 0.1608 |
| | 0.5% | 3.8835 | 3.8417 | | 0.1637 |
| | 1.0% | 3.9028 | 3.8304 | | 0.1663 |
| | 1.5% | 3.9222 | 3.8197 | | 0.1690 |
| | 2.0% | 3.9415 | 3.8090 | | 0.1724 |
| | 2.5% | 3.9608 | 3.7992 | | 0.1732 |
| | 3.0% | 3.9801 | 3.7898 | | 0.1767 |
| | 3.5% | 3.9994 | 3.7799 | | 0.1782 |
| | 4.0% | 4.0188 | 3.7711 | | 0.1807 |
| Fully optimized | -4.0% | 3.7096 | 4.0351 | 0.1383 [001] | 0.2307 [001] |
| | -3.5% | 3.7290 | 4.0066 | 0.1184 [001] | 0.2197 [001] |
| | -3.0% | 3.7483 | 3.9806 | 0.0981 [001] | 0.2088 [001] |
| | -2.5% | 3.7676 | 3.9565 | 0.0769 [001] | 0.1971 [001] |
| | -2.0% | 3.7869 | 3.9343 | 0.0525 [001] | 0.1849 [001] |
| | -1.5% | 3.8062 | 3.9153 | 0.0240 [001] | 0.1724 [001] |
| | -1.0% | 3.8256 | 3.8991 | | 0.1599 [001] |
| | -0.5% | 3.8449 | 3.8852 | | 0.1457 [001] |
| | 0.0% | 3.8642 | 3.8718 | | 0.1315 [001] |
| | 0.5% | 3.8835 | 3.8414 | 0.0249 [110] | 0.1646 [110] |
| | 1.0% | 3.9028 | 3.8287 | 0.0795 [110] | 0.1673 [110] |
| | 1.5% | 3.9222 | 3.8161 | 0.1114 [110] | 0.1704 [110] |
| | 2.0% | 3.9415 | 3.8026 | 0.1373 [110] | 0.1744 [110] |
| | 2.5% | 3.9608 | 3.7891 | 0.1610 [110] | 0.1790 [110] |
| | 3.0% | 3.9801 | 3.7758 | 0.1823 [110] | 0.1836 [110] |
| | 3.5% | 3.9994 | 3.7623 | 0.2022 [110] | 0.1891 [110] |
| | 4.0% | 4.0188 | 3.7489 | 0.2211 [110] | 0.1947 [110] |

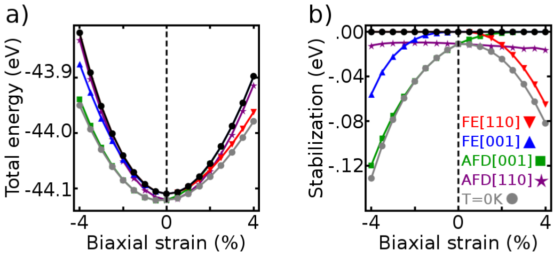


FIG. 1: a) DFT-LDA total energy in VASP of optimized STO structures under biaxial strain perpendicular to [001]. b) Difference in total energy between paraelectric tetragonal STO and these same structures.

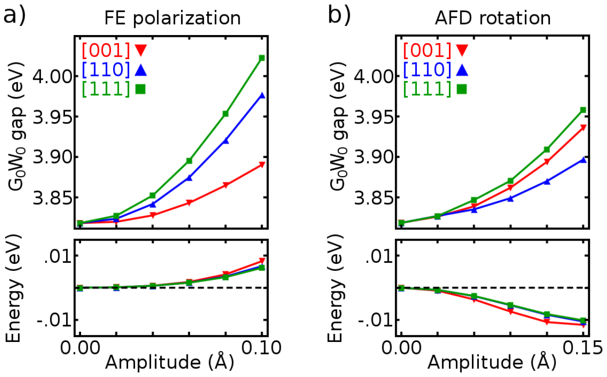


FIG. 2: $G_0W_0$ gaps (top) of STO structures in which a) FE polarization modes and b) AFD rotation modes are frozen in. Per-formula-unit DFT-LDA structural energies relative to cubic STO are also shown (bottom). FE amplitudes are expressed as average relative translations of Ti and O atoms, while AFD amplitudes are expressed as average translations of O atoms. AFD rotations refer to $[001] = a^0a^0c^-$, $[110] = a^-a^-c^0$, and $[111] = a^-a^-a^-$ in Glazer notation.

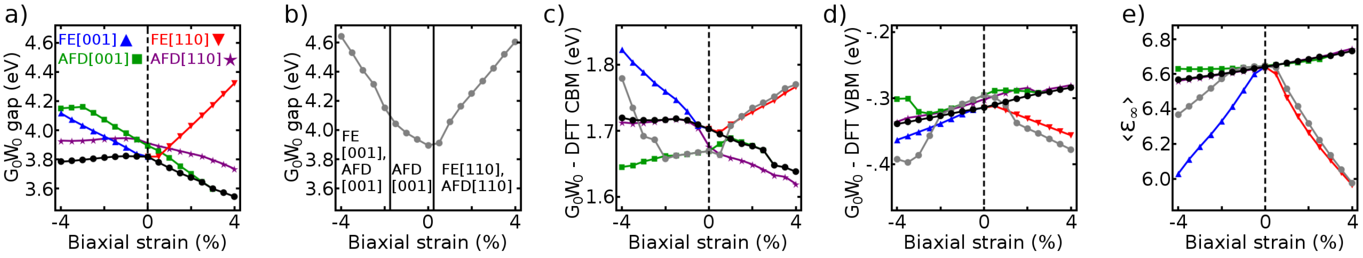


FIG. 3: a) $G_0W_0$ gaps of STO structures under biaxial strain perpendicular to [001], optimized in DFT-LDA with individual ferroic distortions. b) $G_0W_0$ gaps of fully optimized, strained STO structures, computed at zero temperature. $G_0W_0$ corrections to DFT-LDA c) CBM and d) VBM. e) Electronic contribution to the long-wave dielectric constant averaged over the three dimensions (i.e., trace of the dielectric tensor divided by three). $G_0W_0$ corrections are sufficiently constant that they do not qualitatively change DFT-LDA trends, and their small variations reflect changes in screening.

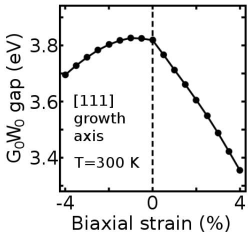


FIG. 4: a) $G_0W_0$ gaps of STO using free energy minimized structures at 300 K under biaxial strain perpendicular to [111]. All structures are paraelectric.
